# Supplementary material for: Deep Visual Geo-localization Benchmark
Source: arXiv:2204.03444 source file (2023-06-09)
Supplement: Supplementary file 2 [file supplementary.tex]

% % CVPR 2022 Paper Template
% % based on the CVPR template provided by Ming-Ming Cheng (https://github.com/MCG-NKU/CVPR_Template)
% % modified and extended by Stefan Roth (stefan.roth@NOSPAMtu-darmstadt.de)

% \documentclass[10pt,twocolumn,letterpaper]{article}

% %%%%%%%%% PAPER TYPE  - PLEASE UPDATE FOR FINAL VERSION
% % \usepackage[review]{cvpr}      % To produce the REVIEW version
% \usepackage{cvpr}              % To produce the CAMERA-READY version
% %\usepackage[pagenumbers]{cvpr} % To force page numbers, e.g. for an arXiv version

% % Include other packages here, before hyperref.
% \usepackage[accsupp]{axessibility}  % Improves PDF readability for those with disabilities.
% \usepackage{graphicx}
% \usepackage{amsmath}
% \usepackage{amssymb}
% \usepackage{booktabs}
% % Other packages
% \usepackage{multirow}


% % It is strongly recommended to use hyperref, especially for the review version.
% % hyperref with option pagebackref eases the reviewers' job.
% % Please disable hyperref *only* if you encounter grave issues, e.g. with the
% % file validation for the camera-ready version.
% %
% % If you comment hyperref and then uncomment it, you should delete
% % ReviewTempalte.aux before re-running LaTeX.
% % (Or just hit 'q' on the first LaTeX run, let it finish, and you
% %  should be clear).
% \usepackage[pagebackref,breaklinks,colorlinks]{hyperref}


% % Support for easy cross-referencing
% \usepackage[capitalize]{cleveref}
% \crefname{section}{Sec.}{Secs.}
% \Crefname{section}{Section}{Sections}
% \Crefname{table}{Table}{Tables}
% \crefname{table}{Tab.}{Tabs.}


% %%%%%%%%% PAPER ID  - PLEASE UPDATE
% \def\cvprPaperID{3658} % *** Enter the CVPR Paper ID here
% \def\confName{CVPR}
% \def\confYear{2022}


% %%%%%%%%% COMMENTS AND OTHER STUFF
% \newcommand{\gb}[1]{{\color{red}{[GB:#1]}}}  %comment
% \newcommand{\gbt}[1]{{\color{red}{#1}}} %coloured text
% \newcommand{\gcs}[1]{{\color{magenta}{[GCS:#1]}}}  %comment
% \newcommand{\gcst}[1]{{\color{magenta}{#1}}} %coloured text
% \newcommand{\cm}[1]{{\color{blue}{[CM:#1]}}}  %comment
% \newcommand{\cmt}[1]{{\color{blue}{#1}}} %coloured text
% \newcommand{\rim}[1]{{\color{cyan}{[RM:#1]}}}  %comment
% \newcommand{\rimt}[1]{{\color{cyan}{#1}}} %coloured text
% \newcommand{\ts}[1]{{\color{blue}{[TS:#1]}}}  %comment

% \newcommand{\gbr}[1]{}
% \newcommand{\gcsr}[1]{}
% \newcommand{\tsr}[1]{}
% \newcommand{\rimr}[1]{}
% \newcommand{\cmr}[1]{}

% %\renewcommand{\gb}[1]{}
% %\renewcommand{\gcs}[1]{}
% %\renewcommand{\ts}[1]{}
% %\renewcommand{\rim}[1]{}
% %\renewcommand{\cm}[1]{}
% %\renewcommand{\gt}[1]{}

% \newcommand{\myparagraph}[1]{\vspace{4pt}\noindent\textbf{#1.}}
% \begin{document}

% %%%%%%%%% TITLE - PLEASE UPDATE
% \title{Deep Visual Geo-localization Benchmark:\\Supplementary Material}

% \author{%
%   \textbf{Gabriele Berton} \\
%   Politecnico di Torino\\
%   \and
%   \textbf{Riccardo Mereu}\\
%   Politecnico di Torino\\
%   \and
%   \textbf{Gabriele Trivigno}\\
%   Politecnico di Torino\\
%   \and
%   \textbf{Carlo Masone}\\
%   CINI
%   %Consorzio Interuniversitario Nazionale per l'Informatica\\
%   \and
%   \textbf{Gabriela Csurka}\\
%   NAVER LABS Europe\\
%   \and
%   \textbf{Torsten Sattler}\\
%   %Czech Institute of Informatics,\\ Robotics and Cybernetics, \\
%   CIIRC, Czech Technical \\ 
%   University in Prague
%   \and
%   \textbf{Barbara Caputo}\\
%   Politecnico di Torino\\
% }

% \maketitle
% %%%%%%%%% Introduction
% This supplementary material contains additional information that could not fit within the main paper due to a lack of space:
% \begin{itemize}
%     \item[-] Section~\ref{sec:supp_datasets} describes in detail the datasets used in the benchmark.
%     \item[-] Section~\ref{sec:supp_software} explains the organization of the open-source software that implements the benchmark.
%     \item[-] Section~\ref{sec:supp_ext_results} provides extended results and discussions for the experiments presented in the main paper.
%     \item[-] Section~\ref{sec:supp_additional_experiments} contains additional experiments and discussions that complement the tests presented in the main paper.
% \end{itemize}


% %%%%%%%%% BODY TEXT
% \input{./supp_chapters/supp1_benchmark}
% \input{./supp_chapters/supp2_software}
% \input{./supp_chapters/supp3_results}
% \input{./supp_chapters/supp4_new_experiments}
% \input{./supp_chapters/supp5_conclusion}

% %%%%%%%%% REFERENCES
% {\small
% \bibliographystyle{ieee_fullname}
% \bibliography{benchmark}
% }

% \end{document}
